# Supplementary material for: Jellium and Cell Model for Titratable Colloids with Continuous Size Distribution
Source: arXiv:1807.09542 ancillary file (2018-07-25)
Supplement: Supplementary file 1 [file Supporting_Information.pdf]

# Jellium and cell model applied to polydisperse charged colloids: Supporting Information

Guillaume Bareigts* and Christophe Labbez†

*ICB UMR 6303 CNRS, Univ. Bourgogne Franche-Comté, FR-21000 Dijon, France*

(Dated: July 25, 2018)

* guillaume.bareigts@u-bourgogne.fr

† christophe.labbez@u-bourgogne.fr

**CONTENTS**


S1. Numerical resolution of the Poisson-Boltzmann Equation 2

S2. Analytical expression for $A_0$ 3

S3. Analytical expression for $A$ at $\Phi = 0$ 4

S4. Bare surface charge densities for monodisperse dispersions 5

S5. Screening in HS40 silica suspensions 6

S6. Osmotic pressures of the PRJM 7

References 7


## S1. NUMERICAL RESOLUTION OF THE POISSON-BOLTZMANN EQUATION

Here we describe how the Poisson–Boltzmann equation (PBE) in the CM and the RJM is solved. For a spherical particle of radius $R$ with a surface potential $\psi_0$ placed in a spherical cell of radius $R_c$ the PBE and boundary conditions write

$$\begin{cases} \frac{\partial^2\psi}{\partial r^2} + \frac{1}{r}\frac{\partial\psi}{\partial r} + 4\pi\lambda_B \left[\sum_{i=1}^{n_I} z_i c_{s,i} \exp(-z_i\psi(r)) + \xi(r)\right] = 0 \\ \psi(R) = \psi_0 \\ \frac{\partial\psi}{\partial r}\Big|_{r=R_c} = 0, \end{cases} \tag{S1}$$

This system of equations is numerically solved using an “in house” code based on Newton Gauss–Seidel iterations[1]. In brief, Eq. S1 is discretized into $N+2$ intervals of length $h$:

$$F_i(\boldsymbol{\psi}) = 0 \quad \forall i = 1, \ldots, N, \tag{S2}$$

with $\boldsymbol{\psi}$ the vector $(\psi_0\psi_1 \ldots \psi_{N+1})$ and

$$F_i(\boldsymbol{\psi}) = \frac{\psi_{i+1} + \psi_{i-1} - 2\psi_i}{h^2} + \frac{\psi_{i+1} - \psi_{i-1}}{hr_i} + 4\pi\lambda_B \left[\sum_{j=1}^{n_I} z_j c_{s,j} \exp(-z_j\psi_i) + \xi(r)\right], \tag{S3}$$

for all $i = 1, \ldots, N$. The boundary condition at the edge of the cell ($r_{N+1} = R_c$) is

$$\psi_{N+1} = \psi_N \tag{S4}$$

The system of algebraic nonlinear equations defined by Eq. S2 is then solved iteratively. A Newton Gauss–Seidel step $p+1$ updates $\boldsymbol{\psi}$ at step $p$, $\boldsymbol{\psi}^{(p)}$, to

$$\begin{cases} \psi_i^{(p+1)} = \psi_i^{(p)} - \frac{F_i(\boldsymbol{\psi}^{(p)})}{\left.\frac{\partial F_i(\boldsymbol{\psi})}{\partial \psi_i}\right|_{\boldsymbol{\psi}=\boldsymbol{\psi}^{(p)}}} & \forall i = 1, \dots, N \\ \psi_{N+1}^{(p+1)} = \psi_N^{(p+1)} & , \end{cases} \tag{S5}$$

with

$$\frac{\partial F_i(\boldsymbol{\psi})}{\partial \psi_i} = -\frac{2}{h^2} - 4\pi\lambda_B \sum_{j=1}^{n_I} z_j^2 c_{s,j} \exp(-z_j\psi_i) \tag{S6}$$

See Ref. [1], Eq. 19.6.43. This is repeated until

$$\sum_{i=1}^{N} F_i(\boldsymbol{\psi})^2 <= N\epsilon^2, \tag{S7}$$

where $\epsilon$ is a given tolerance. The step in Eq. S5 can be slightly improved by replacing $\psi_{i-1}^{(p)}$ by $\psi_{i-1}^{(p+1)}$, as far as the latter is already calculated for the previous index $i-1$. Note that for the RJM, the cell radius is chosen large enough such as a bulk solution exists within the cell.

The source code for the polydisperse RJM and CM, along with examples, are available at this address: `https://github.com/guibar64/polypbren`.

## S2. ANALYTICAL EXPRESSION FOR $A_0$

In this section a detailed development of the analytical expression for the slope, $A_0$, of the linear variation of the bare surface charge density of spherical colloids with $(\kappa R)^{-1}$ and $(\kappa R)^{-1} \ll 1$ is given.

Carvalho *et al* [2] showed that for colloids with a small dimensionless curvature, $\zeta = (\kappa R)^{-1} \ll 1$, their bare surface charge density, $\sigma$, is related to the diffuse layer potential, $\psi_d = \psi(R)$, (see Eq. A14 in [2]) as follow

$$\frac{4\pi\lambda_B\sigma_{bare}}{\kappa_{res}} = 2\sinh\left(\frac{\psi_d}{2}\right) + 4\zeta\tanh\left(\frac{\psi_d}{4}\right) \tag{S8}$$

At the planar limit ($\zeta = 0$) the above equation reduces to

$$\frac{4\pi\lambda_B\sigma_{plane}}{\kappa} = 2\sinh\left(\frac{\psi_{d,plane}}{2}\right), \tag{S9}$$

where $\sigma_{plane}$ and $\psi_{d,plane}$ are the bare charge density and the diffuse potential of the plane.

A first-order Taylor development of Eq. S8 about $\zeta$, with $\zeta \ll 1$, gives

$$\frac{4\pi\lambda_B\sigma_{plane}}{\kappa}(1+A_0\zeta) = 2\sinh(\frac{\psi_{d,plane}}{2}) + \zeta\left[4\tanh\left(\frac{\psi_{d,plane}}{4}\right) + \cosh\left(\frac{\psi_{d,plane}}{2}\right)\left(\frac{\partial\psi_d}{\partial\zeta}\right)_{\zeta=0}\right], \quad \text{(S10)}$$

where $A_0 = \left(\frac{\partial\sigma_{plane}}{\partial\zeta}\right)_{\zeta=0}$, which combined with Eq. S9 yields

$$\frac{4\pi\lambda_B\sigma_{plane}}{\kappa_{res}}A_0 = 4\tanh\left(\frac{\psi_{d,plane}}{4}\right) + \cosh\left(\frac{\psi_{d,plane}}{2}\right)\left(\frac{\partial\psi_d}{\partial\zeta}\right)_{\zeta=0} \quad \text{(S11)}$$

After some algebra, one further finds

$$\frac{4\pi\lambda_B\sigma_{plane}}{\kappa}A_0 = 4\tanh\left(\frac{\psi_{d,plane}}{4}\right) + \cosh\left(\frac{\psi_{d,plane}}{2}\right)\left[\frac{C\kappa\lambda_{Stern}\sigma_{d,plane}}{q_s} - \frac{1}{q_s}\left(\frac{1}{1-\alpha_{plane}} + C\sigma_{plane}\right)A_0\right] \quad \text{(S12)}$$

where $C = 4\pi\lambda_B\lambda_{Stern}$ is the capacitance of the Stern layer and $\alpha_{plane}$ is the fraction of deprotonated sites of the plane. Indeed,

$$\begin{aligned}\frac{\partial\psi_d}{\partial\zeta} &= \left(\frac{\partial F(\sigma,\zeta)}{\partial\zeta}\right)_\sigma + \left(\frac{\partial F(\sigma,\zeta)}{\partial\sigma}\right)_\zeta\left(\frac{\partial\sigma}{\partial\zeta}\right) \\ &= \frac{C\kappa\lambda_{Stern}\sigma}{q_s} - \frac{1}{q_s}\left(\frac{1}{1-\alpha} + C\sigma\right)A,\end{aligned} \quad \text{(S13)}$$

where

$$F(\sigma,\zeta) = \frac{1}{q_s}\left[\ln(10)(\mathrm{pH} - \mathrm{p}K_a) - \ln\left(\frac{\alpha}{1-\alpha}\right) - \frac{C}{1+\lambda_{Stern}/R}\right], \quad \text{(S14)}$$

*c.f.* Eq. 33 of the main manuscript.

From equation S12 the final expression of $A_0$ can be found which reads

$$A_0 = \frac{\frac{1}{\cosh^2(\psi_{d,plane}/4)} + \frac{C\sigma_{plane}\kappa\lambda_{Stern}}{2q_s\tanh(\psi_{d,plane}/2)}}{1 + \frac{1/(1-\alpha_{plane})+C\sigma_{plane}}{2q_s\tanh(\psi_{d,plane}/2)}} \quad \text{(S15)}$$

## S3. ANALYTICAL EXPRESSION FOR $A$ AT $\Phi = 0$

Here we give a detailed development for the analytical expression of $A$, i.e. $\partial\sigma^*/\partial(\kappa^* R)^{-1}$, in the infinite dilution limit, $\Phi = 0$.

From the work of Aubouy *et al* [3] derived from the exact analytical solution of the PBE arround a charged spherical colloid in the diluted limit obtained by Shkel *et al* [4], one can show

$$\begin{cases} \sigma^* = \frac{\kappa\gamma}{\pi\lambda_B} + \frac{2\gamma}{4\pi R\lambda_B}\left(5 - \frac{\gamma^4+3}{\gamma^2+1}\right) \\ \gamma = \sqrt{1+x^2} - x \\ x = \frac{\kappa + \frac{1}{R}}{2\pi\lambda_B\sigma} \end{cases} \tag{S16}$$

$\sigma^*$ can be re-expressed in a more convenient way as

$$\sigma^* = \frac{\kappa\gamma}{\pi\lambda_B}\left[1 + \frac{1}{2\kappa R}\left(5 - \frac{\gamma^4+3}{\gamma^2+1}\right)\right] \tag{S17}$$

In the limit of infinitely large particle, $R \to \infty$, one can notice that as $x$ (Eq.S16) reduces to $x = \frac{\kappa}{2\pi\lambda_B\sigma}$, the prefactor on the right-hand side of Eq. S17 is nothing but the expression of the effective charge of a planar surface, $\sigma^*_{plane}$ [5]. For sufficiently large particle radius, Eq. S17 then writes

$$\sigma^* = \sigma^*_{plane}\left[1 + \frac{1}{2\kappa R}\left(5 - \frac{\gamma^4+3}{\gamma^2+1}\right)\right] \tag{S18}$$

One then finds in the infinite dilution limit the analytical expression for $A$, by identification with Eq. 37 of the main manuscript, which reads

$$A(\Phi = 0) = \frac{1}{2}\left(5 - \frac{\gamma^4+3}{\gamma^2+1}\right) \tag{S19}$$

At saturation, $\gamma \to 1$ and the latter takes the value $A^{sat}(\Phi = 0) = 3/2$.

## S4. BARE SURFACE CHARGE DENSITIES FOR MONODISPERSE DISPERSIONS

Figure S1 gives the bare surface charge density of a monodisperse silica suspension (radius 8 nm) against volume fraction at several pH, calculated with the CM and the RJM. As for

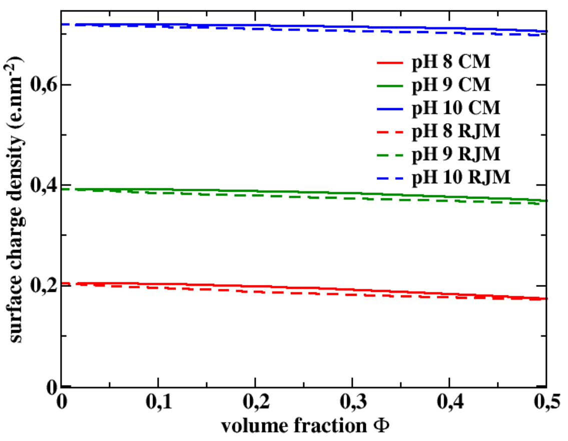


FIG. S1. Bare surface charge density $\sigma_{bare}$ versus volume fraction, Φ, of particles of radius 8 nm in a monodisperse silica suspension at various pH calculated with the CM (full lines), and the RJM (dashed lines).

polydisperse suspensions (Fig. 2 in the main article), $\sigma_{bare}$ increases with pH and decreases with volume fraction. Both models give close results.

## S5. SCREENING IN HS40 SILICA SUSPENSIONS

Fig. S2 compares, in the case of HS40 silica dispersions, the relative effective inverse screening length $\kappa_{eff}/\kappa_{res}$ when accounting or not for the charge regulation or polydispersity. In this case of relatively low polydispersity, the screening length and, thus the pressure is found to be unaffected by the charge regulation and only slightly by the polydispersity.

## S6. OSMOTIC PRESSURES OF THE PRJM

Fig. S3 compares the experimental equations of state of the HS40 and TM50 silica dispersions[6] with the micro-ion pressure calculated with the polydisperse renormalized jellium model at various bulk concentrations of monovalent salt and pH 9. In general the RJM is found to give a bad description of the equation of states of the HS40 and TM50

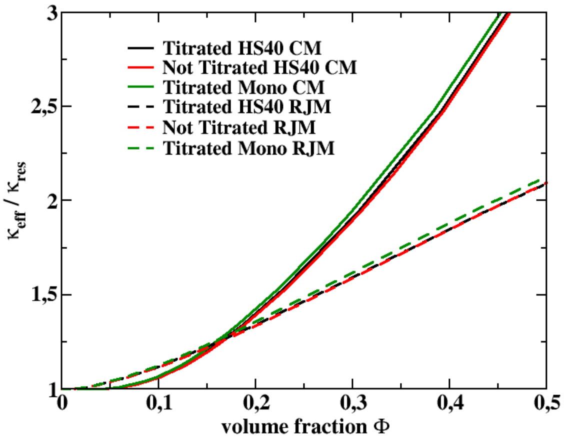


FIG. S2. Relative effective inverse screening length, $\kappa^*/\kappa$, of the HS40 silica suspension in comparison with that of a monodisperse silica suspension with $R = \langle R_{\rm HS40} \rangle$ and a non titrating colloidal suspension with the same particle distribution as the HS40. In the latter, the charge density of all particles is set equal to that of a planar silica surface in the same bulk conditions. The dispersions are in equilibrium with a bulk solution containing 5mM of 1-1 salt and at pH 9. HS40 with titration (black), HS40 without titration (red), Monodisperse 8nm with titration (green). The results are computed with the CM (full lines) and the RJM (dashed lines).

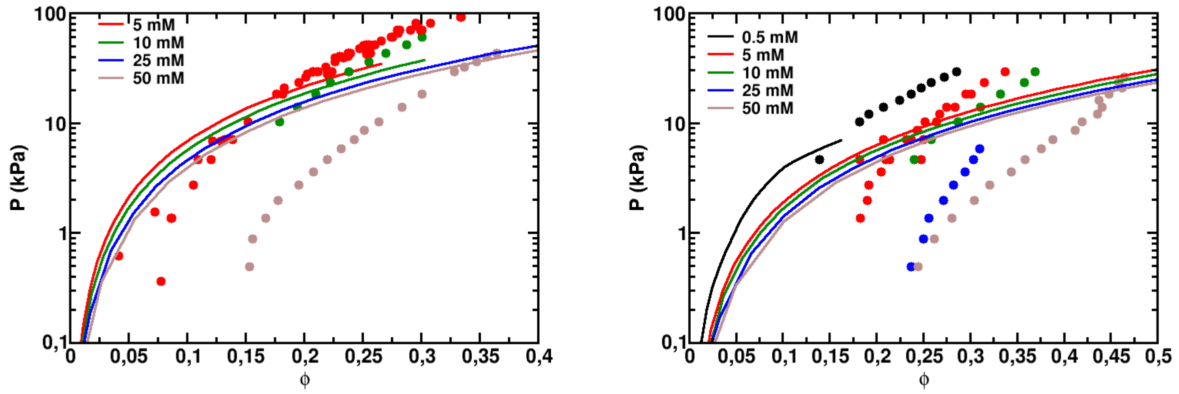


(a) (b)

FIG. S3. Experimental equation of state for the (a) HS40 and (b) TM50 silica dispersions in comparison with the micro-ion pressure calculated by the polydisperse renormolized jellium model at various bulk concentrations of monovalent salt and pH 9.

silica dispersions at finite salt concentrations.


[1] William Press, Saul Teukolsky, William Vetterling, and Brian Flannery, *Numerical Recipes in Fortran: The Art od Scientific Computing*, 2nd ed., edited by Cambridge University Press, Vol. 1 (1992).

[2] Sidney J. de Carvalho, Ralf Metzler, and Andrey G. Cherstvy, "Critical adsorption of polyelectrolytes onto planar and convex highly charged surfaces: The nonlinear Poisson–Boltzmann approach," New J. Phys. **18**, 083037 (2016).

[3] Miguel Aubouy, Emmanuel Trizac, and Lydéric Bocquet, "Effective charge versus bare charge: An analytical estimate for colloids in the infinite dilution limit," J. Phys. A: Math. Gen. **36**, 5835 (2003).

[4] Irina A. Shkel, Oleg V. Tsodikov, and M. Thomas Record, "Complete Asymptotic Solution of Cylindrical and Spherical Poisson-Boltzmann Equations at Experimental Salt Concentrations," J. Phys. Chem. B **104**, 5161–5170 (2000).

[5] Lydéric Bocquet, Emmanuel Trizac, and Miguel Aubouy, "Effective charge saturation in colloidal suspensions," J. Chem. Phys. **117**, 8138–8152 (2002).

[6] Lucas Goehring, Joaquim Li, and Pree-Cha Kiatkirakajorn, "Drying paint: From micro-scale dynamics to mechanical instabilities," Phil. Trans. R. Soc. A **375**, 20160161 (2017).
